# Supplementary material for: SafeDrug: Dual Molecular Graph Encoders for Recommending Effective and Safe Drug Combinations
Source: arXiv:2105.02711 source file (2022-07-17)
Supplement: Supplementary file 1 [file appendix.tex]

\appendix
	
\section{Detailed Calculation of Metrics}
To provide more information about how we evaluate the model, we specify the detailed calculation of metrics used in Section~5.1. We already present the definition of DDI measurement in the main text, in this section, we show the calculation of Jaccard coefficient (Jaccard), F1-score (F1) and precision recall area under curve (PRAUC).

We use $\mathbf{m}_j^{(t)}$ to denote the target drug recommendation at the $t$-th visit of patient $j$, and $\hat{\mathbf{m}}_j^{(t)}$ is the estimated multi-hot drug vector.

\paragraph{Jaccard.} The Jaccard coefficient for patient $j$ at the $t$-th visit is calculated by 

\begin{equation}
    Jaccard_j^{(t)} = \frac{|\{i:~\mathbf{m}_{j,i}^{(t)}=1\}\cap \{i:~\hat{\mathbf{m}}_{j,i}^{(t)}=1\}|}{|\{i:~\mathbf{m}_{j,i}^{(t)}=1\}\cup \{i:~\hat{\mathbf{m}}_{j,i}^{(t)}=1\}|},
\end{equation}
and the Jaccard coefficient for one patient $j$ is by taking the average over his visits ($V_j$ is the total number of visits of patient $j$),
\begin{equation}
    Jaccard_j = \frac{1}{V_j}\sum_{t=1}^{V_j}Jaccard_j^{(t)},
\end{equation}
while the overall Jaccard coefficient of the test data is by taking further average over all patients ($P$ is the total number of patients),
\begin{equation}
    Jaccard = \frac{1}{P}\sum_{j=1}^{P}Jaccard_j,
\end{equation}
In the main text, we report only the overall Jaccard coefficient.

\paragraph{F1.} The F1 score is calculated by the harmonic mean of precision and recall. For patient $j$ at the $t$-th visit, the Precision, Recall, F1 are calculated by
\begin{equation}
    Precision_j^{(t)} = \frac{|\{i:~\mathbf{m}_{j,i}^{(t)}=1\}\cap \{i:~\hat{\mathbf{m}}_{j,i}^{(t)}=1\}|}{ |\{i:~\hat{\mathbf{m}}_{j,i}^{(t)}=1\}|}
\end{equation}
\begin{equation}
    Recall_j^{(t)} = \frac{|\{i:~\mathbf{m}_{j,i}^{(t)}=1\}\cap \{i:~\hat{\mathbf{m}}_{j,i}^{(t)}=1\}|}{ |\{i:~{\mathbf{m}}_{j,i}^{(t)}=1\}|}
\end{equation}
\begin{equation}
    F1_j^{(t)} = \frac{2}{\frac{1}{Precision_j^{(t)}}+\frac{1}{Recall_j^{(t)}}}
\end{equation}
The F1 score for one patient $j$ is by taking the average over his visits,
\begin{equation}
    F1_j = \frac{1}{V_j}\sum_{t=1}^{V_j}F1_j^{(t)},
\end{equation}
while the overall F1-score of the test data is by taking further average over all patients,
\begin{equation}
    F1 = \frac{1}{P}\sum_{j=1}^{P}F1_j,
\end{equation}
In the main text, we report only the overall F1-score.

\paragraph{PRAUC.} To compute a PRAUC, we actually treat the drug recommendation as an information retrieval problem. The precision-recall area under curve (PRAUC) for patient $j$ at the $t$-th visit is calculated by 

\begin{align}
    PRAUC_j^{(t)} &= \sum_{k=1}^{|\mathcal{M}|}Precision(k)_j^{(t)}\Delta Recall(k)_j^{(t)},\notag\\
    \Delta Recall(k)_j^{(t)} &= Recall(k)_j^{(t)} - Recall(k-1)_j^{(t)},
\end{align}
where $k$ is the rank in the sequence of the retrieved drugs, $|\mathcal{M}|$ is the number of retrieved documents, $Precision(k)_j^{(t)}$ is the precision at cut-off $k$ in the ordered retrieval list, and $\Delta Recall(k)_j^{(t)}$ is the change in recall from items $k-1$ to $k$. This metric is implemented by the function ``sklearn.metrics.average\_precision\_score" from
\textit{scikit-learn} package.

The PRAUC for one patient $j$ is by taking the average over his visits,
\begin{equation}
    PRAUC_j = \frac{1}{V_j}\sum_{t=1}^{V_j}PRAUC_j^{(t)},
\end{equation}
while the overall PRAUC of the test data is by taking further average over all patients,
\begin{equation}
    PRAUC = \frac{1}{P}\sum_{j=1}^{P}PRAUC_j,
\end{equation}
In the main text, we report only the overall PRAUC.
